# Supplementary material for: An Efficient Training Approach for Very Large Scale Face Recognition
Source: arXiv:2105.10375 source file (2022-03-03)
Supplement: Supplementary file 1 [file sm.tex]

% \clearpage

% To provide more specific analysis of our proposed F$^2$C, we introduce why we design F$^2$C and more ablation studies in appendix section.

% \subsection{Why Dual Data-Loaders}
% As mentioned in our manuscript, we design dual data-loader to improve the update efficiency of DCP parameters.
% We analyze the different influences between identity-based and instance-based loaders as follows.
% Let $M$ denote batch size, $n_{ID}$ be the total number of identities given the dataset, $k_{min}$ ($k_{max}$) as the minimum (maximum) number of images for one person in the dataset, $\bar{k}$ be the average number of images per identity.
% Here the shape of DCP mentioned in the main paper is $C \times K \times D$.
% $C$ is the size of DCP. $D$ represents feature dimension.
% The total images of given dataset can be denoted as $\bar{k}n_{ID}$.
% We use the number of iterations to count the update speed.
% % maybe "count" is better than "represent"
% \begin{itemize}
% \item If we only use instance-based loader, the update speed of identities' centers $\in[\frac{\bar{k}n_{ID}}{Mk_{max}}, \frac{\bar{k}n_{ID}}{Mk_{min}}]$. So only using instance-based loader may lead to following problems. 1. If the number of identities is very imbalanced, the update speed of the identities' centers that have rare number of images is too slow. 2. If we sample $M$ images that belong to $M$ different identities, the DCP may have no positive samples for this iteration. In this case, cross entropy, which is crucial for classification, cannot be calculated.

% \item If we only use identity-based loader, we can obtain the fastest update speed ($\frac{n_{ID}}{M}$) of each identity.
% However, identity-based loader re-sample identities that have rare number of images too many times, so it needs to use about $\frac{k_{max}}{k_{min}}$ times more iterations than instance-based loader to sample all images from the dataset.
% Further, the sample probabilities for each instance of identities with rich intra-class images are too low, the identity-based loader can not sample plenty of intra-class images during the training phase.

% \item Using the dual data-loader can inherit the benefits from instance-based and identity-based loaders.
% First, dual data-loader provides appropriate ratios between positive and negative images, which is very important for face recognition.
% Second, dual data-loader keeps high update efficiency (speed) of identities' centers and various intra-class images.
% \end{itemize}

% \subsection{Exploring the influence of ratios between dual data-loader.}

% We set the ratio of the size between instance-based and identity-based loaders as 1:1 by default.
% To further explore the influence of the ratios within dual data-loader, we show the experiments in Table \ref{tab:7}.
% We utilize ResNet-50 as backbone to train MS-Celeb-1M dataset.
% We find that the default ratio within dual data-loader achieves the highest results on most datasets, especially on challenging IJBC and MegaFace.


% \begin{table*}[htp]
%     \centering
%     \caption{Evaluation the ratios between dual data-loader.
%     All models are trained on MS-Celeb-1M using ResNet-50.
%     The TPR@FPR metric is used for IJBC and MegaFace.}
%     \resizebox{\textwidth}{15mm}{
%     \begin{tabular}{@{}ccccccccccc@{}}
% \toprule
% Ins.L & ID.L  &AGEDB&LFW &CALFW &CPLFW &SLFW &YTF   &CFP &IJBC(1e-4) & MegaFace(1e-6) \\ 
	
% 	%&&&&\multicolumn{3}{l}{\textbf{Training on MS-Celeb-1M}}\\
% 	\midrule
% 	0 & 1 &97.40 &99.77 &95.22  &89.75 &99.18 &97.92  &98.20 &91.75 &93.65\\
% % 	upper-boundary &94.46  &85.03 &98.72 &95.88  &83.94 &97.63\\
% 	1 & 0 &96.60 &99.68 &94.67  &88.17 &98.92 &97.15  &97.41 &92.06 &92.74\\
% 	1 & 1 &\textbf{97.83} &99.50 &\textbf{95.58}  &\textbf{90.58} &99.45 &\textbf{98.16}  &\textbf{98.46} &\textbf{94.91} &\textbf{96.74}\\
% 	2 & 1 &97.87 & \textbf{99.88} &90.33  &90.33 &\textbf{99.57} &97.80  &98.30 &94.21 &96.43\\
% 	1 & 2 &96.97 &99.75 &88.32  &88.32 &98.93 &97.72  &97.80 &90.80 &90.56\\
% \bottomrule
% \label{tab:7}
% \end{tabular}} 
% \end{table*}

% \subsection{Ablation of $L_{ce}$ and $L_{cos}$}


% \begin{algorithm*}[htp]
% \caption{DCP: PyTorch-like Pseudocode}
% \label{alg:code}
% % \algcomment{
% \textbf{Notes}: Both \textbf{lru.view} and \textbf{lru.get} will return the oldest position if lru is full or new empty position when the cache is not full.
% The difference is \textbf{lru.view} won't change the internal state of lru while the latter changes.
% It's used to decide the position that gallery features will be placed to.
% % }
% \definecolor{codeblue}{rgb}{0.25,0.5,0.5}
% \definecolor{codekw}{rgb}{0.85, 0.18, 0.50}
% \begin{lstlisting}[language=python]
% # p_data: input to probe net
% # g_data: input to gallery net
% # lru: least recently used cache-algorithm.
% # dcp: dynamic class pool, shape is 2 * pool_size * feat_dim
% # add_margin: implements forward methods of AM,Arc,MV etc.
% def forward(p_data, g_data, probe_label, gallery_label):
%     mask = torch.zeros(pool_size, 1)
%     p = probe_net(p_data) # get probe features
%     with torch.no_grad():  # no gradient to gallery
%         momentum_update_gallery() # update the gallery net
%         g = gallery_net(g_data) # get gallery features.
%     rows = []  # determine the position in dcp
%     cols = [] # determine the position in dcp
%     ones_idx = set([])
%     queue_position_dict = {}
%     for i in range(pool_size):
%         queue_position_dict[i] = 0
%     for i, gl in enumerate(gallery_label): 
%         if gl not in lru:
%             idx = lru.get(gl) 
%             rows.append(0) 
%             cols.append(idx)
%             queue_position_dict[idx] = 1
%         else:
%             idx = lru.get(gl)
%             rows.append(queue_position_dict[idx])
%             cols.append(idx)
%             ones_idx.add(idx)
%             queue_position_dict[idx] = (queue_position_dict[idx] + 1) % 2
%     r = torch.LongTensor(rows).cuda(g.device)
%     c = torch.LongTensor(cols).cuda(g.device)
%     with torch.no_grad():
%         dcp[r, c] = g # gallery features are used as class center.
%     fake_labels = [] # dynamically decide probe label
%     for pl in probe_label:
%         fake_labels.append(lru.view(pl)) 
%     label = torch.LongTensor(fake_labels).cuda(p.device)
%     cos_theta1 = F.linear(p, dcp[0])
%     mask_idx = torch.LongTensor(list(ones_idx))
%     mask[mask_idx, 0] = 1
%     with torch.no_grad():
%         weight = mask * dcp[1] + (1 - mask) * dcp[0]
%     cos_theta2 = F.linear(p, weight)
%     loss = add_margin(cos_theta1, label) + add_margin(cos_theta2, label)
%     return loss

% \end{lstlisting}
% \end{algorithm*}



% \subsection{The specific update strategy of DCP}

% We introduce the Dynamic Class Pool (DCP) as a substitute for FC layer. For clarity, the pseudocode of DCP is described in Algorithm \ref{alg:code}.



% \subsection{Ablation Studies using ResNet-50}
% As mentioned in our manuscript, we append the ablation studies using ResNet-50 as backbone. The results are shown in Table \ref{tab:8}, Table \ref{tab:9} and Table\ref{tab:10}, respectively.
% Using dual data-loader and dual nets obtains the highest performance on all datasets.
% Our experiments of K prove that the larger K can provide more reliable center estimation than smaller one. 


% \begin{table}[H]
% \centering
% \caption{Comparison of single or dual data loaders.}
% \label{tab:8}
% % \setlength{\abovecaptionskip}{0.cm}
% \vspace{-0.5em}
% \begin{tabular}{@{}cccc@{}}
% \toprule
% Method  &Small Datasets  &IJBC & MegaFace \\ 
	
% 	%&&&&\multicolumn{3}{l}{\textbf{Training on MS-Celeb-1M}}\\
% 	\midrule
% 	ID.L   &96.70  &91.75 &93.65\\
% 	Ins.L   &96.08  &92.06 &92.74\\
% 	Dua.L  & \textbf{97.07}  & \textbf{94.91} & \textbf{96.74}\\

% \bottomrule
% \end{tabular} 
% \end{table}


% \begin{table}[H]
% \centering
% \caption{Comparison of single net or dual nets.}
% \label{tab:9}
% % \setlength{\abovecaptionskip}{0.cm}
% \vspace{-0.5em}
% \begin{tabular}{@{}ccccccc@{}}
% \toprule
% Method  &SmallDatasets   &IJBC & MegaFace \\ 
	
% 	%&&&&\multicolumn{3}{l}{\textbf{Training on MS-Celeb-1M}}\\
% 	\midrule
% 	Single Net   &95.55  &92.26 &92.98\\
% 	Dual Net   & \textbf{97.07}  & \textbf{94.91} & \textbf{96.74}\\

% \bottomrule
% \end{tabular} 
% \end{table}


% \begin{table}[H]
% \centering
% \caption{Comparison of the number of K.}
% \label{tab:10}
% % \setlength{\abovecaptionskip}{0.cm}
% \vspace{-0.5em}
% \begin{tabular}{@{}cccc@{}}
% \toprule
% Num. of K  &Small Datasets  &IJBC & MegaFace \\ 
	
% 	%&&&&\multicolumn{3}{l}{\textbf{Training on MS-Celeb-1M}}\\
% 	\midrule
% 	1   &96.58  &94.38 &96.49\\
% 	2   & \textbf{97.07}  & \textbf{94.91} & \textbf{96.74} \\

% \bottomrule
% \end{tabular} 
% \end{table}
